# Supplementary material for: Universal Domain Adaptation for Robust Handling of Distributional Shifts in NLP
Source: arXiv:2310.14849 source file (2023-10-23)
Supplement: Supplementary file 1 [file appendix_different_thresholds.tex]

\begin{figure*}[t]
% \begin{figure}[t]
    \centering
    \begin{subfigure}{0.23\textwidth}
        \includegraphics[width=\textwidth]{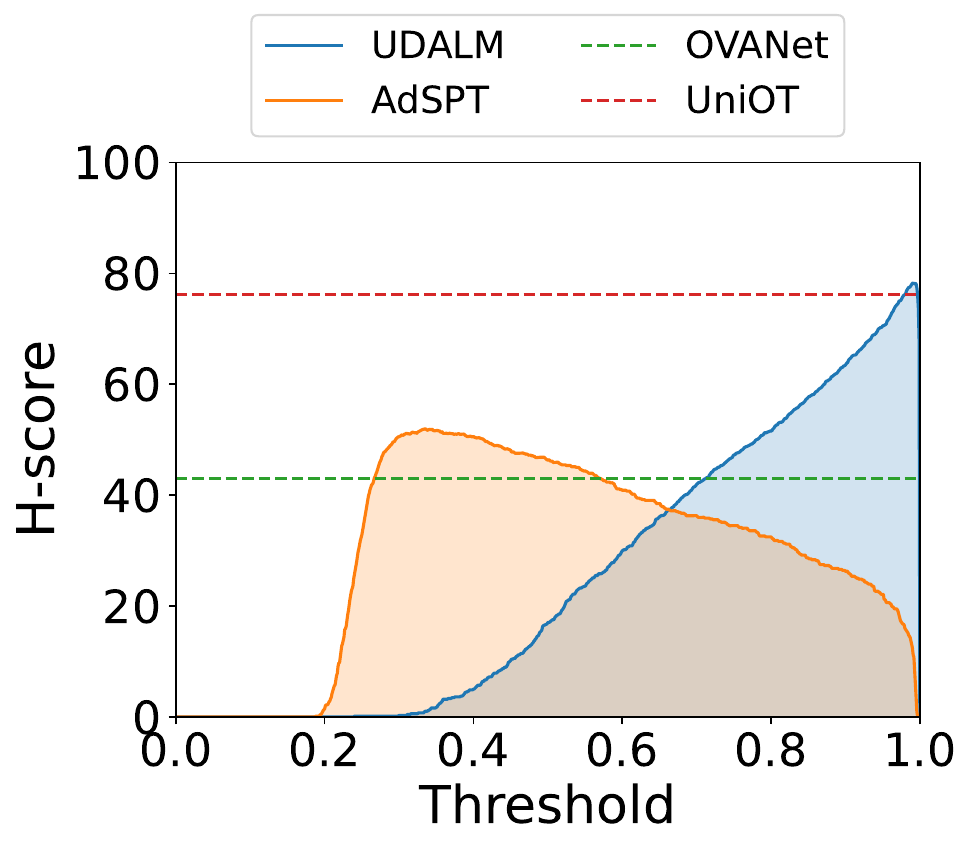}
        \caption{CLINC-150}
        \label{figure:appendix_different_thresholds_clinc}
    \end{subfigure}
    \hfill
    \begin{subfigure}{0.23\textwidth}
        \includegraphics[width=\textwidth]{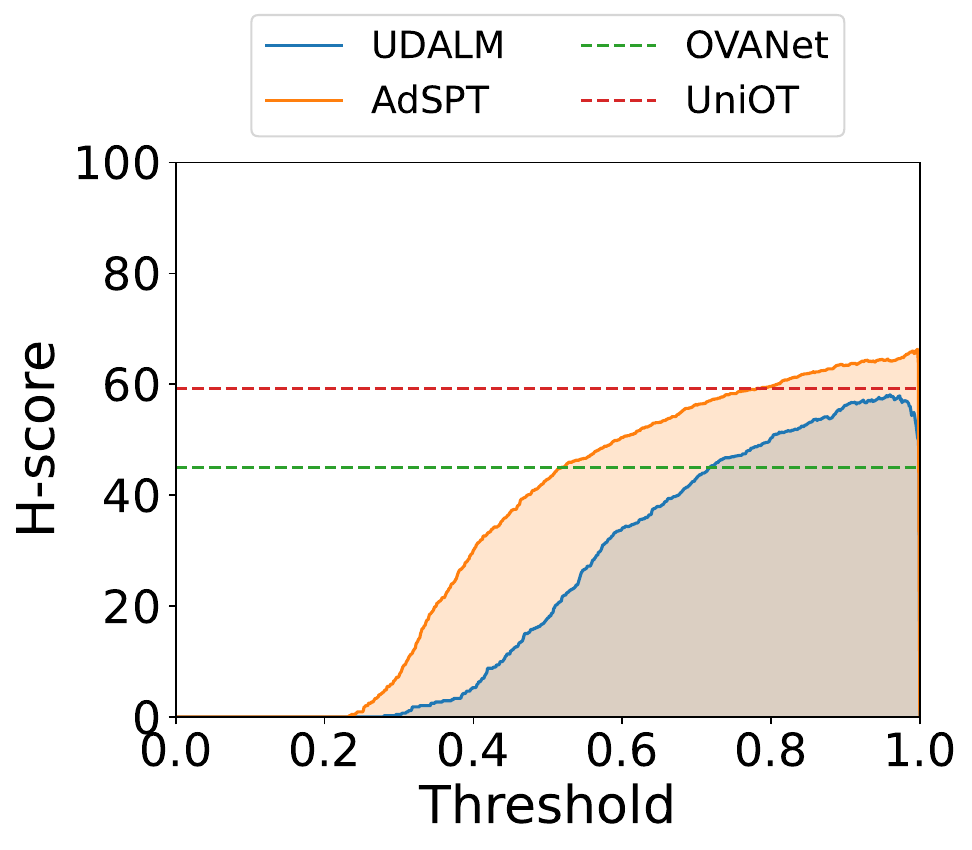}
        \caption{Huffpost (2012 $\rightarrow$ 2013)}
        \label{figure:appendix_different_thresholds_2013}
    \end{subfigure}
    \hfill
    \begin{subfigure}{0.23\textwidth}
        \includegraphics[width=\textwidth]{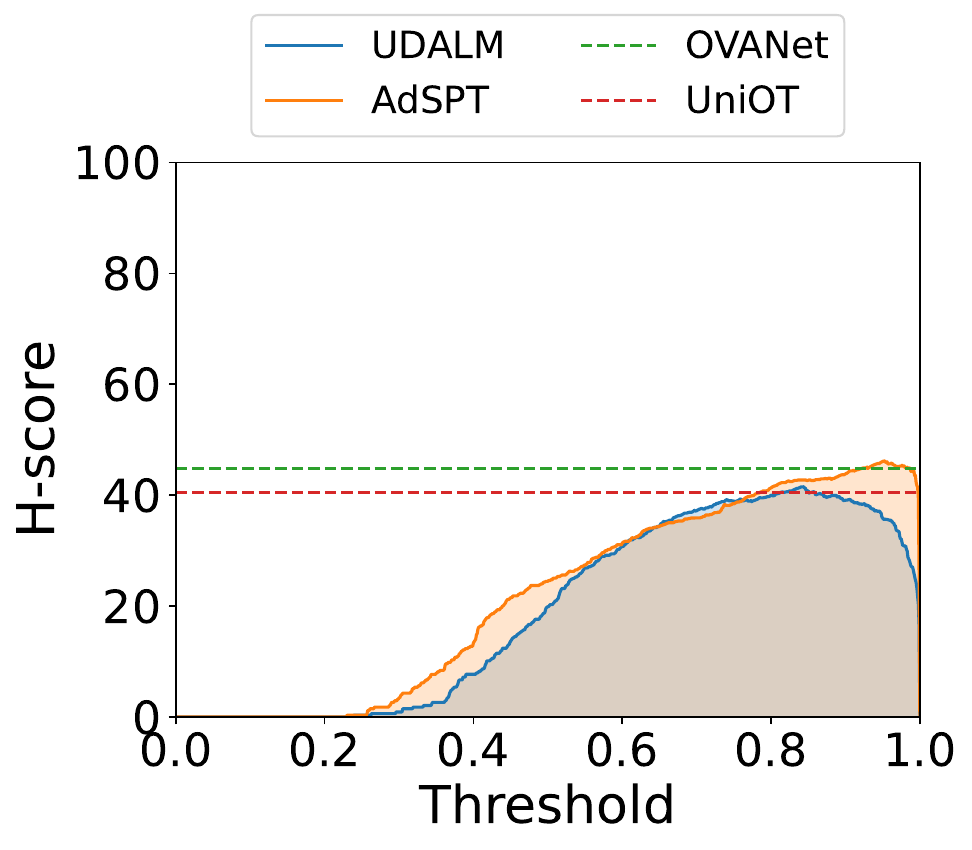}
        \caption{Huffpost (2012 $\rightarrow$ 2014)}
        \label{figure:appendix_different_thresholds_2014}
    \end{subfigure}
    \hfill
    \begin{subfigure}{0.23\textwidth}
        \includegraphics[width=\textwidth]{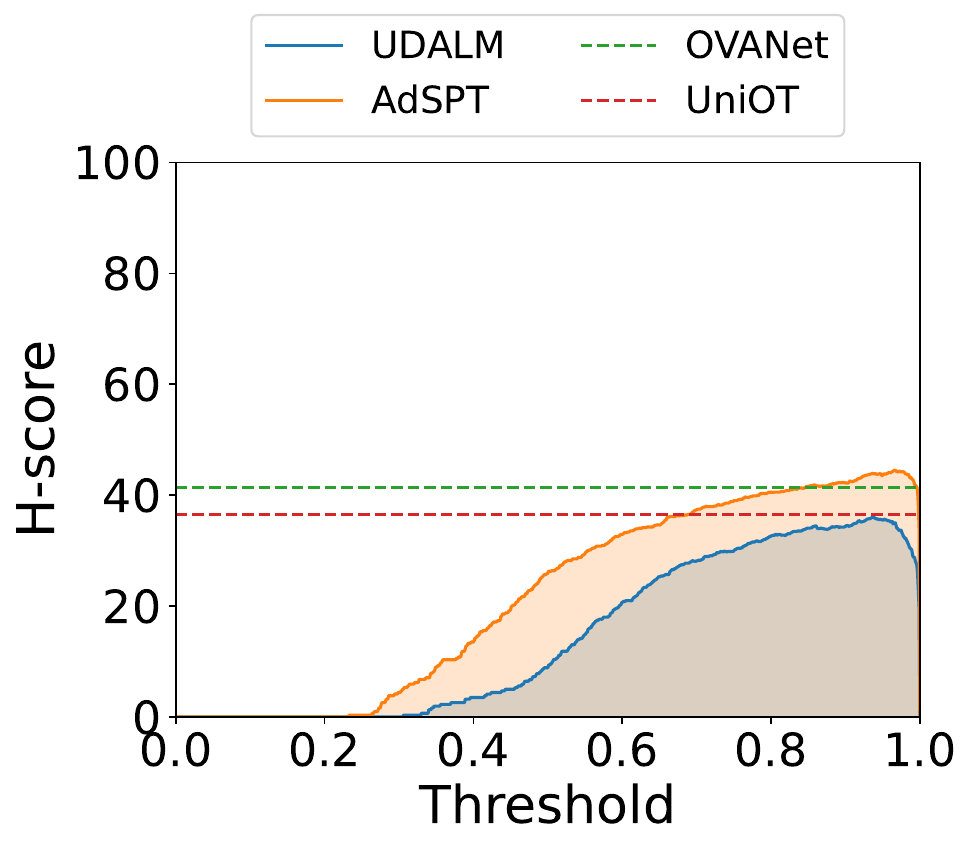}
        \caption{Huffpost (2012 $\rightarrow$ 2015)}
        \label{figure:appendix_different_thresholds_2015}
    \end{subfigure}
    \hfill
    \begin{subfigure}{0.23\textwidth}
        \includegraphics[width=\textwidth]{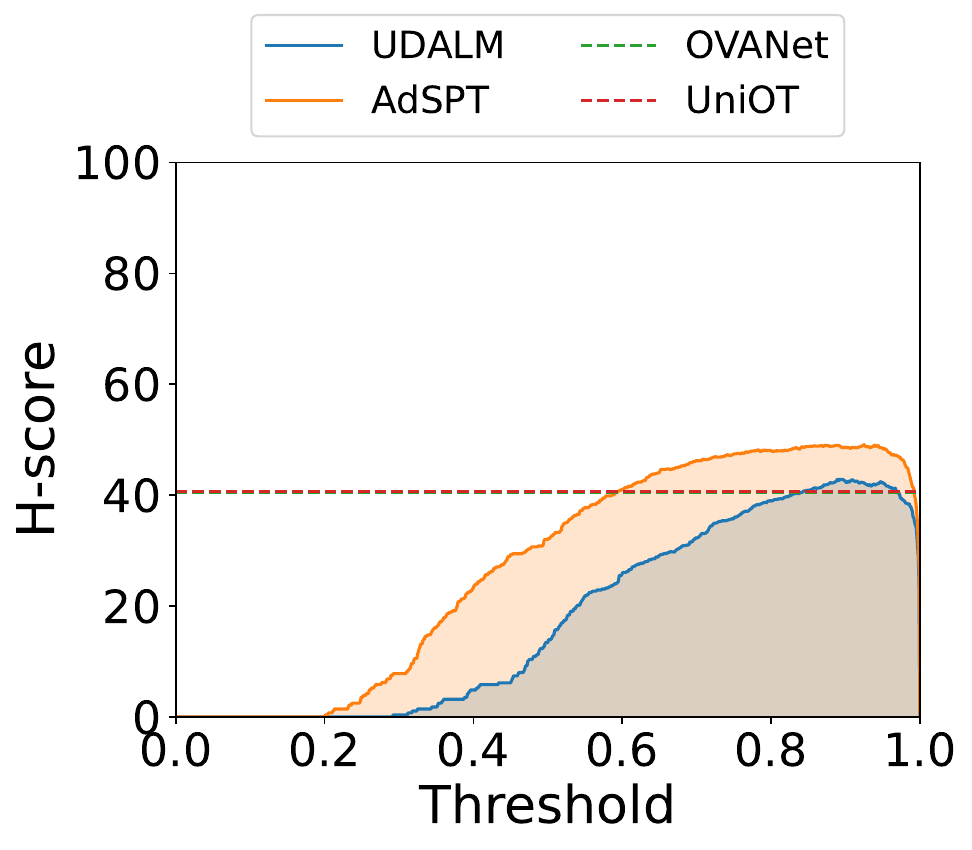}
        \caption{Huffpost (2012 $\rightarrow$ 2016)}
        \label{figure:appendix_different_thresholds_2016}
    \end{subfigure}
    \hfill
    \begin{subfigure}{0.23\textwidth}
        \includegraphics[width=\textwidth]{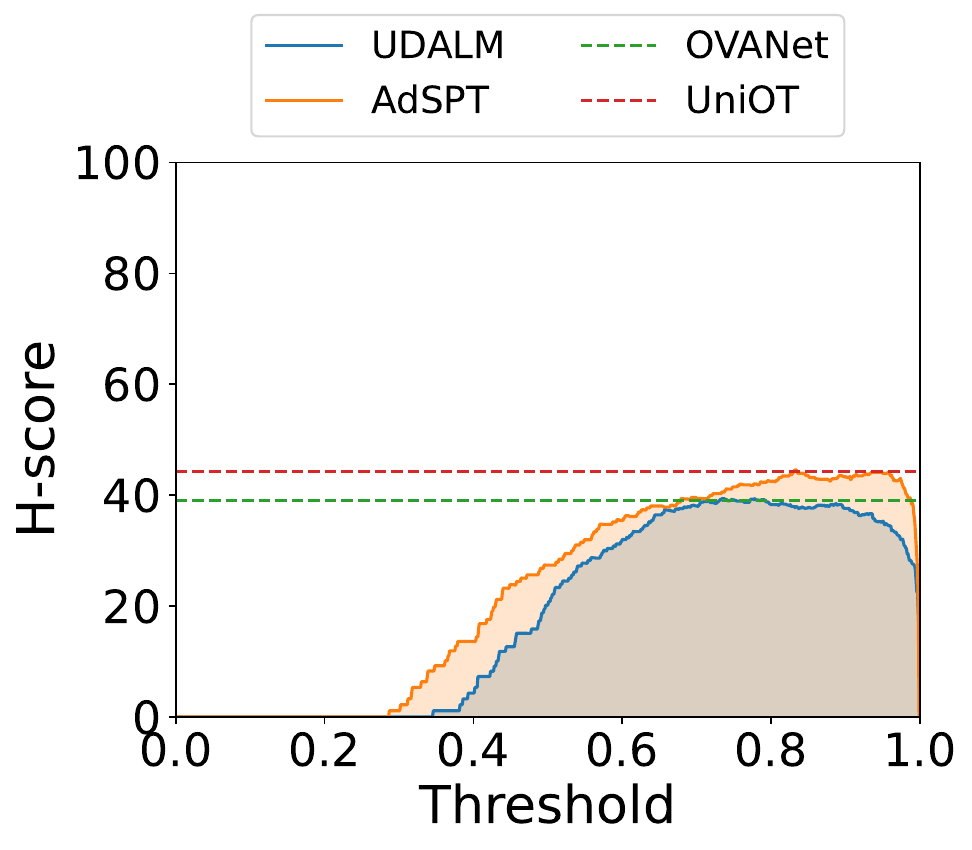}
        \caption{Huffpost (2012 $\rightarrow$ 2017)}
        \label{figure:appendix_different_thresholds_2017}
    \end{subfigure}
    \hfill
    \begin{subfigure}{0.23\textwidth}
        \includegraphics[width=\textwidth]{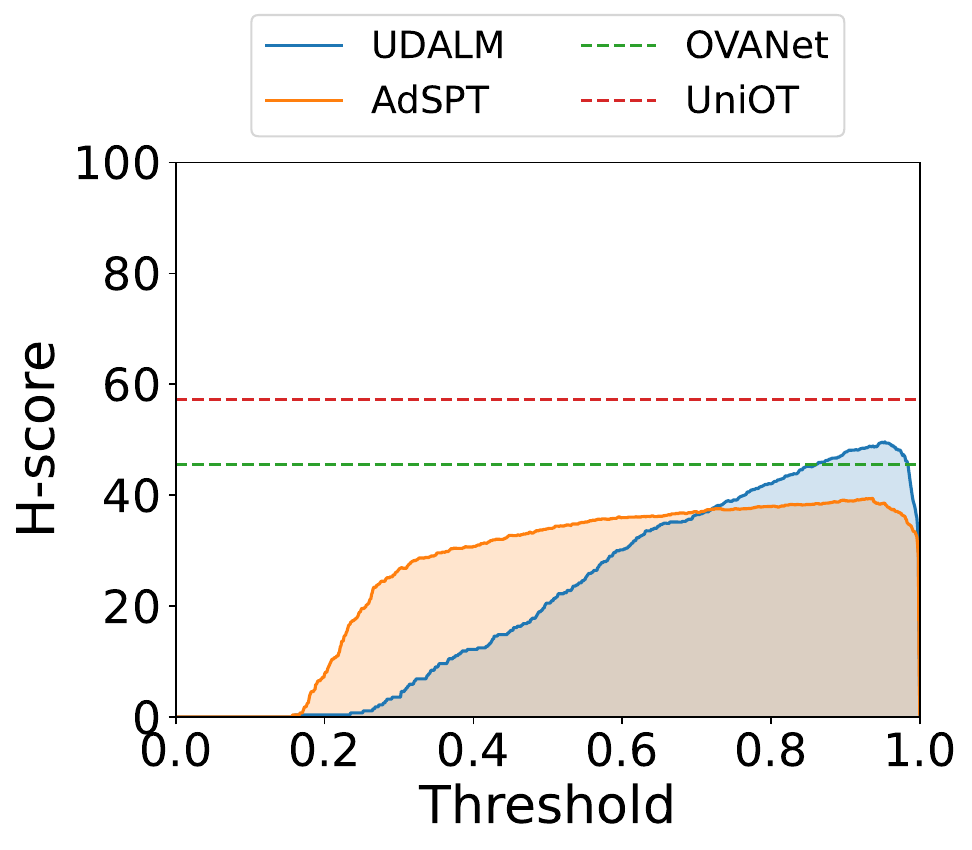}
        \caption{MASSIVE}
        \label{figure:appendix_different_thresholds_massive}
    \end{subfigure}
    \hfill
    \begin{subfigure}{0.23\textwidth}
        \includegraphics[width=\textwidth]{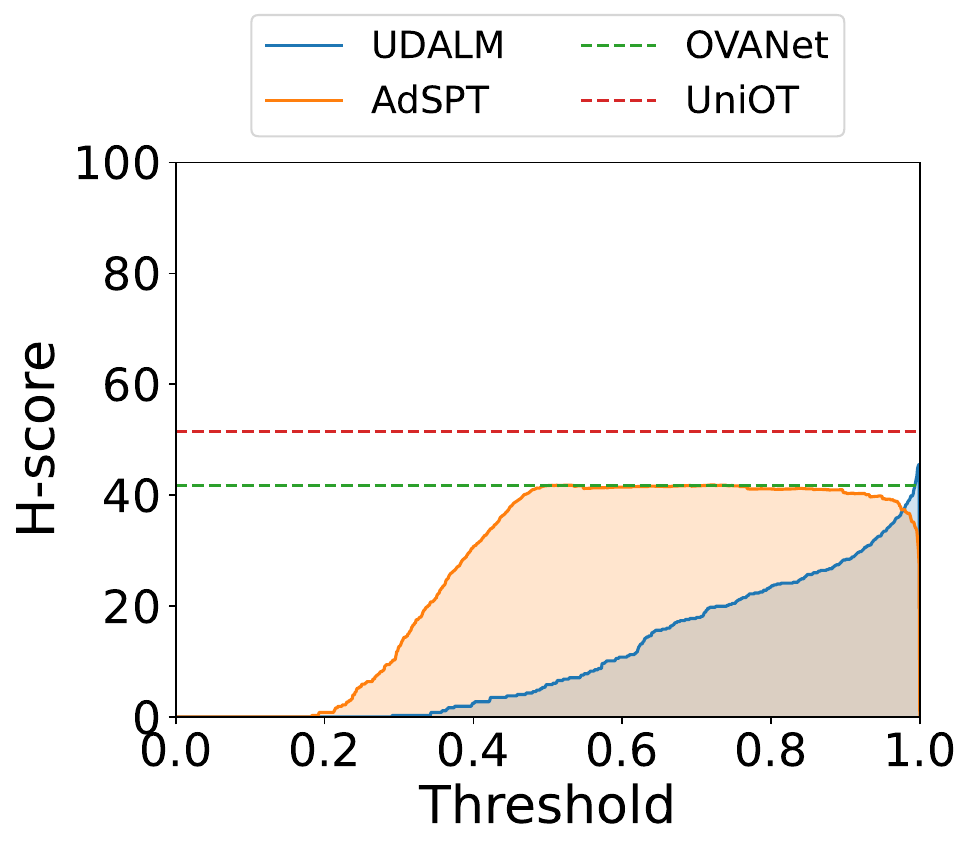}
        \caption{Amazon}
        \label{figure:appendix_different_thresholds_amazon}
    \end{subfigure}

    \caption{
        H-score performance with different threshold values applied to CDA methods for all the proposed datasets.
        The H-score of UniDA methods are visualize as a horizontal line.
        % In easy or moderate adaptation scenario, CDA exhibit the potential to outperform UniDA methods. 
        % With an optimal threshold, CDA methods are capable of outperforming UniDA in certain circumstances.
    }
    \label{figure:appendix_different_thresholds}
% \end{figure}
\end{figure*}
